# Supplementary material for: PingPong: Packet-Level Signatures for Smart Home Device Events
Source: arXiv:1907.11797 source file (2020-02-10)
Supplement: Supplementary file 1 [file appendix.tex]

\begin{table*}[htb!]
  \centering
  \begin{center}
  { \footnotesize
  %\small
  \begin{tabular}{| p{13mm} | p{14mm} | c | c | c | c | c | c | c | c | c |}
    \hline
        & & & & & \multicolumn{6}{ c |}{\textbf{Matching (Per 100 Events)}}\\
    \cline{6-11}
        \textbf{Device} & \textbf{Event} & \textbf{Signature} & \textbf{Comm.} & \textbf{Duration (ms)} & \multicolumn{4}{ c |}{\textbf{No Defense}} & \multicolumn{2}{ c |}{\textbf{STP+VPN}} \\
	\cline{6-11}
        & & & & \textbf{Min./Avg./Max.} & \textbf{WAN} & \textbf{FPR} & \textbf{Wi-Fi} & \textbf{FPR} & \textbf{WAN} & \textbf{FPR}\\
        & & & & & \textbf{Snif.} & & \textbf{Snif.} & & \textbf{Snif.} & \\
    \hline
    	\multicolumn{11}{| c |}{\textbf{Plugs}}\\
	\hline
        Amazon & ON & \textbf{S1:} S-[443-445] & \devicecloudcomm & 1,232 / 2,465 / 4,537 & 98 & 0 & 99 & 0 & 99 & 0\\
        plug & & \textbf{S2:} C-1099 S-235 & & & & & & & & \\
	\cline{2-3}
        & OFF & \textbf{S1:} S-[444-446] & & & & & & & & \\
        & & \textbf{S2:} C-1179 S-235 & & & & & & & & \\
        & & \textbf{S3:} C-1514 C-103 S-235 & & & & & & & & \\
	\hline
        WeMo & ON/OFF & \textbf{S1:} PH-259 PH-475 D-246 & \phonedevicecomm & 33 / 42 / 134 & - & - & 100 & 0 & - & - \\
        plug$\ast$ & & & & & & & & & & \\
	\hline
        WeMo & ON/OFF & \textbf{S1:} PH-259 PH-475 D-246 & \phonedevicecomm & 32 / 39 / 97 & - & - & 99 & 0 & - & - \\
        Insight & & & & & & & & & & \\
        plug$\ast$ & & & & & & & & & & \\
	\hline
        TP-Link & ON & \textbf{S1:} C-556 S-1293 & \devicecloudcomm & 75 / 85 / 204 & 99 & 0 & - & - & 98 & 3 \\
    \cline{2-3}
        plug$\bullet$ & OFF & \textbf{S1:} C-557 S-[1294-1295] & & & & & & & & \\
    \cline{2-11}
        & ON & \textbf{S1:} PH-112 D-115 & \phonedevicecomm & 225 / 325 / 3,328 & - & - & 99 & 0 & - & - \\
        & & \textbf{S2:} C-556 S-1293 & \& & & & & & & & \\
	\cline{2-3}
	     & ON & \textbf{S1:} PH-112 D-115 & \devicecloudcomm & & & & & & & \\
        & & \textbf{S2:} C-557 S-[1294-1295] & & & & & & & & \\
	\hline
        D-Link plug & ON/OFF & \textbf{S1:} S-91 S-1227 C-784 & \devicecloudcomm & 4 / 1,194 / 8,060 & 95 & 0 & 95 & 0 & 95 & 0 \\
        & & \textbf{S2:} C-1052 S-647 & & & & & & & & \\
    \cline{2-11}
    	& ON & \textbf{S1:} C-[1109-1123] S-613 & \phonecloudcomm & 35 / 41 / 176 & 98 & 0 & 98 & 0 & 98 & 0\\
    \cline{2-3}
        & OFF & \textbf{S1:} C-[1110-1124] S-613 & & & & & & & & \\
    \hline
        SmartThings & ON & \textbf{S1:} C-699 S-511 & \phonecloudcomm & 335 / 537 / 2,223 & 92 & 0 & 92 & 0 & 92 & 0\\
        plug & & \textbf{S2:} S-777 C-136 & & & & & & & & \\
	\cline{2-3}
        & OFF & \textbf{S1:} C-700 S-511 & & & & & & & & \\
        & & \textbf{S2:} S-780 C-136 & & & & & & & & \\
    \hline
    	\multicolumn{11}{| c |}{\textbf{Light Bulbs}}\\
	\hline
        Sengled & ON & \textbf{S1:} S-[217-218] C-[209-210] & \devicecloudcomm & 4,304 / 6,238 / 8,145 & 97 & 0 & - & - & 97 & 0\\
        light & & \textbf{S2:} C-430 & & & & & & & & \\
        bulb$\dagger$ & & \textbf{S3:} C-466 & & & & & & & & \\
	\cline{2-3}
        & OFF & \textbf{S1:} S-[217-218] C-[209-210] & & & & & & & & \\
        & & \textbf{S2:} C-430 & & & & & & & & \\
        & & \textbf{S3:} C-465 & & & & & & & & \\
	\cline{2-11}
        & ON & \textbf{S1:} C-211 S-1063 & \phonecloudcomm & 4,375 / 6,356 / 9,132 & 93 & 0 & 97 & 0 & 96 & 1\\
        & & \textbf{S2:} S-1277 & & & & & & & & \\
	\cline{2-3}
        & OFF & \textbf{S1:} C-211 S-1063 S-1276 & & & & & & & & \\
	\cline{2-11}
        & Intensity & \textbf{S1:} S-[216-220] & \devicecloudcomm & 16 / 74 / 824 & 99 & 2 & - & - & 99 & 5\\
        & & C-[208-210] & & & & & & & & \\
	\cline{2-11}
        & Intensity & \textbf{S1:} C-[215-217] & \phonecloudcomm & 3,916 / 5,573 / 7,171 & 99 & 0 & 99 & 0 & 98 & 2 \\
        & & S-[1275-1277] & & & & & & & & \\
	\hline
        Hue light & ON & \textbf{S1:} C-364 & \devicecloudcomm & 11,019 / 12,787 / & - & - & - & - & - & -\\
        bulb$\diamond$ & & \textbf{S2:} D-88 & \& & 14,353 & & & & & & \\
	\cline{2-3}
        & OFF & \textbf{S1:} C-365 & \phonedevicecomm & & & & & & & \\
		& & \textbf{S2:} D-88 & & & & & & & & \\
	\hline
        TP-Link & ON & \textbf{S1:} PH-198 D-227 & \phonedevicecomm & 8 / 77 / 148 & - & - & 100 & 4 & - & - \\
	\cline{2-3}
        light & OFF & \textbf{S1:} PH-198 D-244 & & & & & & & & \\
    \cline{2-11}
        bulb$\ast$ & Intensity & \textbf{S1:} PH-[240-242] D-[287-289] & \phonedevicecomm & 7 / 84 / 212 & - & - & 100 & 0 & - & - \\
    \cline{2-11}
        & Color & \textbf{S1:} PH-317 D-287 & \phonedevicecomm & 6 / 89 / 174 & - & - & 100 & 0 & - & - \\
    \hline
    	\multicolumn{11}{| c |}{\textbf{Thermostats}}\\
	\hline
    	Nest & Fan ON & \textbf{S1:} C-[891-894] S-[830-834] & \phonecloudcomm & 91 / 111 / 1,072 & 93 & 0 & 93 & 1 & 93 & 2 \\
    \cline{2-3}
    	thermostat & Fan OFF & \textbf{S1:} C-[858-860] S-[829-834] & & & & & & & & \\
   	\hline
        Ecobee & HVAC Auto & \textbf{S1:} S-1300 C-640 & \phonecloudcomm & 121 / 229 / 667 & 100 & 0 & 99 & 0 & 99 & 0\\
	\cline{2-3}
        thermostat & HVAC OFF & \textbf{S1:} C-1299 C-640 & & & & & & & & \\
	\cline{2-11}
        & Fan ON & \textbf{S1:} S-1387 C-640 & \phonecloudcomm & 117 / 232 / 1,776 & 100 & 0 & 100 & 0 & 100 & 1\\
	\cline{2-3}
        & Fan Auto & \textbf{S1:} C-1389 C-640 & & & & & & & & \\
    \hline
    	\multicolumn{11}{| c |}{\textbf{Sprinklers}}\\
	\hline
        Rachio & Quick Run & \textbf{S1:} S-267 C-155 & \devicecloudcomm & 1,972 / 2,180 / 2,450 & 100 & 0 & 100 & 0 & 100 & 1\\
	\cline{2-3}
        sprinkler & Stop & \textbf{S1:} C-496 C-155 C-395 & & & & & & & & \\
	\cline{2-11}
        & Standby/ Active & \textbf{S1:} S-299 C-155 C-395 & \devicecloudcomm & 276 / 690 / 2,538 & 100 & 0 & 100 & 0 & 100 & 0\\
    \hline
        Blossom & Quick Run & \textbf{S1:} C-326 & \devicecloudcomm & 701 / 3,470 / 8,431 & 96 & 0 & 96 & 0 & 96 & 3\\
        sprinkler$\ddagger$ & & \textbf{S2:} C-177 S-505 & & & & & & & & \\
	\cline{2-3}
        & Stop & \textbf{S1:} C-326 & & & & & & & & \\
        & & \textbf{S2:} C-177 S-458 & & & & & & & & \\
        & & \textbf{S3:} C-238 C-56 S-388 & & & & & & & & \\
    \cline{2-11}
        & Quick Run & \textbf{S1:} C-649 S-459 C-574 S-507 & \phonecloudcomm & 70 / 956 / 3,337 & 93 & 0 & 93 & 0 & 93 & 0\\
        & & \textbf{S2:} S-[135-139] & & & & & & & & \\
	\cline{2-3}
        & Stop & \textbf{S1:} C-617 S-431 & & & & & & & & \\
    \cline{2-11}
        & Hibernate & \textbf{S1:} C-621 S-493 & \phonecloudcomm & 121 / 494 / 1,798 & 95 & 0 & 93 & 0 & 93 & 1\\
	\cline{2-3}
        & Active & \textbf{S1:} C-622 S-494 & & & & & & & & \\
        & & \textbf{S2:} S-599 C-566 S-554 C-566 & & & & & & & & \\
    \hline
  \end{tabular}
  }
  \end{center}
  %\caption{Smart home devices found to exhibit \phonecloudcomm, \devicecloudcomm, and \phonedevicecomm signatures 
  %	(prefix PH indicates Phone-to-device direction and prefix D indicates Device-to-phone direction;
  %	the duration of each signature is measured from the first packet of 
  %	the first sequence S1 to the last packet of the last sequence Sn).
  %	\label{tab:wan-signatures}}
\end{table*}

\clearpage
\begin{table*}[htb!]
  \centering
  \begin{center}
  { \footnotesize
  %\small
  \begin{tabular}{| p{14mm} | p{14mm} | c | c | c | c | c | c | c | c | c |}
    \hline
        & & & & & \multicolumn{6}{ c |}{\textbf{Matching (Per 100 Events)}}\\
    \cline{6-11}
        \textbf{Device} & \textbf{Event} & \textbf{Signature} & \textbf{Comm.} & \textbf{Duration (ms)} & \multicolumn{4}{ c |}{\textbf{No Defense}} & \multicolumn{2}{ c |}{\textbf{STP+VPN}} \\
	\cline{6-11}
        & & & & \textbf{Min./Avg./Max.} & \textbf{WAN} & \textbf{FPR} & \textbf{Wi-Fi} & \textbf{FPR} & \textbf{WAN} & \textbf{FPR}\\
        & & & & & \textbf{Snif.} & & \textbf{Snif.} & & \textbf{Snif.} & \\
    \hline
    	\multicolumn{11}{| c |}{\textbf{Home Security Devices}}\\
	\hline
        Ring alarm & Arm & \textbf{S1:} S-99 S-254 C-99 & \devicecloudcomm & 275 / 410 / 605 & 98 & 0 & 95 & 0 & 95 & 0\\
        & & S-[181-183] C-99 & & & & & & & & \\
	\cline{2-3}
        & Disarm & \textbf{S1:} S-99 S-255 C-99 & & & & & & & & \\
        & & S-[181-183] C-99 & & & & & & & & \\
    \hline
        Arlo & Stream ON & \textbf{S1:} C-[338-339] S-[326-329] & \phonecloudcomm & 46 / 78 / 194 & 99 & 2 & 98 & 3 & 97 & 4\\
        camera & & C-[364-365] S-[1061-1070] & & & & & & & & \\
        & & \textbf{S2:} C-[271-273] S-[499-505] & & & & & & & & \\
	\cline{2-3}
        & Stream OFF & \textbf{S1:} C-[445-449] S-442 & & & & & & & & \\
	\hline
        D-Link siren & ON & \textbf{S1:} C-1076 S-593 & \phonecloudcomm & 36 / 37 / 65 & 100 & 0 & 98 & 0 & 97 & 0 \\
	\cline{2-3}
        & OFF & \textbf{S1:} C-1023 S-613 & & & & & & & & \\
	\hline
        Kwikset & Lock & \textbf{S1:} C-699 S-511 & \phonecloudcomm & 173 / 395 / 2,874 & 100 & 0 & 100 & 0 & 100 & 0\\
        door & & \textbf{S2:} S-639 C-136 & & & & & & & & \\
	\cline{2-3}
        lock & Unlock & \textbf{S1:} C-701 S-511 & & & & & & & & \\
        & & \textbf{S2:} S-647 C-136 & & & & & & & & \\
    \hline
    	\multicolumn{11}{| c |}{\textbf{Others}}\\
	\hline
        Roomba & Clean & \textbf{S1:} S-[1014-1015] C-105 & \phonecloudcomm & 123 / 2,038 / 5,418 & 91 & 0 & 94 & 0 & 94 & 1\\
        robot$\ddagger$ & & S-432 C-105 & & & & & & & & \\
	\cline{2-3}
        & Back-to- & \textbf{S1:} S-440 C-105 & & & & & & & & \\
        & station & S-[1018-1024] C-105 & & & & & & & & \\
    \hline
    	\multicolumn{5}{| r |}{Average} & 97.05 & 0.18 & 97.48 & 0.32 & 96.77 & 1.09 \\
    \hline
  \end{tabular}
  }
  \end{center}
  \caption{Smart home devices found to exhibit \phonecloudcomm, \devicecloudcomm, and \phonedevicecomm signatures 
  	(prefix PH indicates Phone-to-device direction and prefix D indicates Device-to-phone direction;
  	the duration of each signature is measured from the first packet of 
  	the first sequence S1 to the last packet of the last sequence Sn;
	$\ast$the \wemoplug, \wemoinsightplug, and \tplinkbulb exhibit \phonedevicecomm signatures---these are
	observable only by the Wi-Fi sniffer;
	$\dagger$the \sengledbulb's \devicecloudcomm signatures are sent by the Zigbee hub to the cloud 
	through the Ethernet interface; thus, they are not 	observable by the \wifisniffer;
	$\ddagger$the \roombarobot had a few events missed because the device failed to return 
	to the base station after a back-to-station command at the time the app issued the following 
	clean command; the \blossomsprinkler also had a few events missed because the app reported connection
	lost for some triggers;
	$\bullet$the \tplinkplug's \devicecloudcomm signatures are observable both by the WAN and Wi-Fi sniffers;
	for the Wi-Fi sniffer, there is an additional \phonedevicecomm pair.
	$\diamond$the \huebulb has unique signatures; they consist of a pair, in which
	one is a \devicecloudcomm packet coming from the Zigbee hub to the cloud---this 
	is observable only by the \wansniffer since the hub is an Ethernet device---and 
	the other one is a \phonecloudcomm packet---this is observable only by the \wifisniffer;
	thus we did not use the signatures to perform detection since they partially belong to both adversaries).
  	\label{tab:summary-signatures}}
\end{table*}
